# Supplementary material for: A partition-based similarity for classification distributions
Source: arXiv:2011.06557 source file (2020-11-12)
Supplement: Supplementary file 1 [file appendix.tex]

% \section{Proofs of Theorems  \ref{thm:ats=1=ats}, \ref{thm:non-decreasing}, \ref{thm:consistent_classifier} and \ref{thm:histogram-rules}}\label{app:theorems}


% \begin{theorem}
% $ATS(F, G) \le TS(F,G)$
% \end{theorem}

% \begin{proof}
%   Let $F^S, F^T$ be arbitrary distributions respectively on $\mc{X}\times\{1, \dots, k^S\}$ and $\mc{X}\times\{1, \dots, k^T\}$. Consider $ATS(F^T, F^S)$ and $TS(F^T, F^S)$. Since
%   \begin{align*}
%       \int_{A_S} \mbb{I}\{h^{*}_T(x) = y\}\mbb{I}\{|\psi_{A_S}^{T}| = 1\} dF^{T}_{X} \geq \int_{A_S} \mbb{I}\{h^{*}_T(x) = y\}dF^{T}_{X} 
%   \end{align*}
%   For all $A_S \in \mc{A}_S$ where $\mc{A}_S$ is the optimal partition induced by $F^S$, we have that by summing over $A_S$, we get $TS(F^T,F^S) \geq ATS(F^T, F^S)$, as desired.
% \end{proof}
% \begin{theorem}
% Let $\mc{A}$ be a partition on $\mc{X}$, and let $F^T, F^S \in \mc{F}_{\mc{A}}$, then $TS(F^T, F^S) = TS(F^S, F^T) = 1$.
% \end{theorem}

% \subsection*{Theorem \ref{thm:ats=1=ats}}
% \begin{proof}
%     Assume $F^T, F^S \in \mc{F}_{A}$. Thus $\mc{A}$ is the optimal partition of both $F^T$ and $F^S$. 
    
%     Let $F^T$ have $k^T$ classes and let $F^S$ have $k^S$ classes. We have by definition of adjusted task similarity 
%     \begin{align*}
%         ATS(F^T, F^S) = \sum_{A \in \mc{A}}\max_{y \in \{1, \dots, k^T\}}\int_{A} 
%         \mbb{I}\{h^{*}_T(x) = y\}
%         \cdot
%         \mbb{I}\{|\psi_{A}^{T}| = 1\}
%         dF^{T}_{X}.
%     \end{align*}
%     Examining the term $\mbb{I}\{|\psi_{A}^{T}| = 1\}$,
%     \begin{align*}
%          \mbb{I}\{|\psi_{A}^{T}| = 1\} = \mbb{I}\{|\argmax_{y \in \{1, \hdots, k^{T}\}} \int_{A}
%     \mbb{I}\{h_{T}^{*}(x) = y\} dF^{T}_{X}| = 1\}
%     \end{align*}
%     Since $\mc{A}$ is the optimal partition for $F^T$, we have that $h_T^*$ is constant on $A \in \mc{A}$, say $h_T^* = y_A$. The integral above by is maximized by taking $y$ to be $y_A$, as any other $y$ would make it zero. Thus argmax always has only one element, $y_A$, and the indicator is always equal to one. Thus 
%     \begin{align*}
%         ATS(F^T, F^S) & = \sum_{A \in \mc{A}}\max_{y \in \{1, \dots, k^T
%         \}}\int_{A} 
%         \mbb{I}\{h^{*}_T(x) = y\}
%         \cdot
%         \mbb{I}\{|\psi_{A}^{T}| = 1\}
%         dF^{T}_{X}\\
%         &= \sum_{A \in \mc{A}}\max_{y \in \{1, \dots, k^T\}}\int_{A} \mbb{I}\{h^{*}_T(x) = y\} dF^{T}_{X}
%     \end{align*}
%     By the same argument again, as $\mc{A}$ is the optimal partition for $F^T$ and hence $h^*_T$ is constant on $A$, we get that the indicator is always $1$ as $y$ is taken to be $y_A$, which is the constant value that $h_T^*$ takes on in $A$. Thus 
%      \begin{align*}
%         TS(F^T, F^S) & = 
%         \sum_{A \in \mc{A}}\max_{y \in \{1, \dots, k^T\}}\int_{A} \mbb{I}\{h^{*}_T(x) = y\} dF^{T}_{X} \\
%         & = \sum_{A \in \mc{A}}\int_{A}dF^T_X \\
%         & = 1
%     \end{align*}
%     Since $\mc{A}$ is a partition for $\mc{X}$. Thus $ATS(F^T, F^S) = 1$. By symmetry, $ATS(F^S, F^T) = 1$ also, and so the desired result.
% \end{proof}

% \subsection*{Theorem \ref{thm:non-decreasing}}
% \begin{proof}
%   Assume $F^T, F^S \in \mc{F}_{A}$. Thus $\mc{A}$ is the optimal partition of both $F^T$ and $F^S$. 
    
%     Let $F^T$ have $k^T$ classes and let $F^S$ have $k^S$ classes. We have by definition of task similarity 
%     \begin{align*}
%         TS(F^T, F^S) = \sum_{A \in \mc{A}}\max_{y \in \{1, \dots, k^T\}}\int_{A} 
%         \mbb{I}\{h^{*}_T(x) = y\}
%         dF^{T}_{X}.
%     \end{align*}
%     Since $\mc{A}$ is the optimal partition for $F^T$, we have that $h_T^*$ is constant on $A \in \mc{A}$, say $h_T^* = y_A$. The integral above by is maximized by taking $y$ to be $y_A$, as any other $y$ would make it zero. Thus the indicator is always equal to one, and so
%      \begin{align*}
%         TS(F^T, F^S) & = 
%         \sum_{A \in \mc{A}}\max_{y \in \{1, \dots, k^T\}}\int_{A} \mbb{I}\{h^{*}_T(x) = y\} dF^{T}_{X} \\
%         & = \sum_{A \in \mc{A}}\int_{A}dF^T_X \\
%         & = 1
%     \end{align*}
%     Since $\mc{A}$ is a partition for $\mc{X}$. Thus $TS(F^T, F^S) = 1$. By symmetry, $TS(F^S, F^T) = 1$ also, and so the desired result. 
% \end{proof}

% \subsection*{Theorem \ref{thm:consistent_classifier}}

% \subsection*{Theorem \ref{thm:histogram-rules}}
% \begin{proof}
%   Let $\mc{B}$ be a subpartition of $\mc{A}$ and let $F_{\mc{A}} \in \mc{F}_{\mc{A}}$ and $F_{\mc{B}} \in \mc{F}_{\mc{B}}$. Let $F^T$ be an arbitrary distribution on $\mc{X}\times\{1, \dots, k\}$. 
   
%   Consider now $\Delta = TS(F, F_{\mc{B}}) - TS(F, F_{\mc{A}})$. We would like to show this quantity is greater than or equal to zero, and we get the desired result.
   
%   Since $\mc{B}$ is a subpartition of $\mc{A}$, then every element of $\mc{A}$ is the union of the elements of some subset of $\mc{B}$. Thus let $A \in \mc{A}$ be arbitrary, and let $\mc{B}_{A}$ be such that $A = \bigcup_{B \in \mc{B}_A}B$. Then,
%   \begin{align*}
%     \sum_{B \in \mc{B}_A}
%     \max_{y \in \{1, \dots, k^T\}}
%     \int_{B} 
%         \mbb{I}\{h^{*}_T(x) = y\}
%         dF^{T}_{X}
%         -
%     \max_{y \in \{1, \dots, k^T\}}
%     \int_{A} 
%         \mbb{I}\{h^{*}_T(x) = y\}
%         dF^{T}_{X}.
%   = \\      
%   \sum_{B \in \mc{B}_A}
%     \max_{y \in \{1, \dots, k^T\}}
%     \int_{B} 
%         \mbb{I}\{h^{*}_T(x) = y\}
%         dF^{T}_{X}
%         -      
%     \max_{y \in \{1, \dots, k^T\}}
%     \sum_{B \in \mc{B}_A}
%     \int_{B} 
%         \mbb{I}\{h^{*}_T(x) = y\}
%         dF^{T}_{X}
%   \end{align*}
%   Hence the difference between $TS(F^T, F_\mc{B})$ and $TS(F^T, F_{\mc{A}})$ is simply moving the maximum inside the sum, i.e. maximizing each integral separately rather than maximizing them all simultaneously. Now unless the same $y$ maximizes each integral, in which case the expressions are equal, maximizing the sum yields a quantity smaller than maximizing each summand separately then summing. Hence,
%   \begin{align*}
%         \sum_{B \in \mc{B}_A}
%     \max_{y \in \{1, \dots, k^T\}}
%     \int_{B} 
%         \mbb{I}\{h^{*}_T(x) = y\}
%         dF^{T}_{X} 
%         - 
%         \max_{y \in \{1, \dots, k^T\}}
%     \sum_{B \in \mc{B}_A}
%     \int_{B} 
%         \mbb{I}\{h^{*}_T(x) = y\}
%         dF^{T}_{X} \geq 0
%   \end{align*}
%   Now summing over each $A \in \mc{A}$,
%     \begin{align*}
%         \sum_{A \in \mc{A}}\sum_{B \in \mc{B}_A}
%     \max_{y \in \{1, \dots, k^T\}}
%     \int_{B} 
%         \mbb{I}\{h^{*}_T(x) = y\}
%         dF^{T}_{X} 
%         -
%         \sum_{A \in \mc{A}}\max_{y \in \{1, \dots, k^T\}}
%     \sum_{B \in \mc{B}_A}
%     \int_{B} 
%         \mbb{I}\{h^{*}_T(x) = y\}
%         dF^{T}_{X}
%   \end{align*}
%   Since $\mc{B}$ subpartition of $\mc{A}$ implies that $\mc{B} = \bigcup_{A \in \mc{A}}\mc{B}_{\mc{A}}$. Hence we get
%   \begin{align*}
%      TS(F^T, F_{\mc{B}}) - TS(F^T, F_{\mc{A}}) \geq 0
%   \end{align*}
%   Which is the desired result.
% \end{proof}

% \begin{proof}
%     Assume the conditions in the theorem. Consider the task similarity $TS(F^T, F^S_n)$,
%     \begin{align*}
%          TS(F^{T}, F^{S}) = 
%     \sum_{A_{S} \in \mc{A}_S^*}
%     \max_{y \in \{1, \dots, k^T\}}
%     \int_{A_{S}}
%     \mbb{I}\{h_{T}^{*}(x) = y\} dF^{T}_{X}.
%     \end{align*}
%     In the above integral, we pick some $y_{A_S}$ such that $y_{A_S}$ maximizes $\int_{A_{S}}\mbb{I}\{h_{T}^{*}(x) = y\} dF^{T}_{X}$. In essence we have just defined $h_n$ where $h_n(x) = y_{A_S}$ whenever $x \in A_S$.In other words, $h_n$ takes on the constant value $y_{A_S}$ on each cell $A_S \in \mc{A}_S$. The task similarity then turns into
%     \begin{align*}
%          TS(F^{T}, F^{S}) & = 
%     \sum_{A_{S} \in \mc{A}_S^*}
%     \max_{y \in \{1, \dots, k^T\}}
%     \int_{A_{S}}
%     \mbb{I}\{h_{T}^{*}(x) = y\} dF^{T}_{X} \\
%     & = \sum_{A_S \in \mc{A}_S}\int_{A_S}\mbb{I}(h_T^*(x) = h_n(x))dF^T_X \\
%     & = \int_{\mc{X}}\mbb{I}\{h_T^*(x) = h_n(x)\}dF^T_X
%     \end{align*}
%     Now, $\mc{A}_1, \mc{A}_2, \dots$ inducing a consistent decision rule implies that
%     \begin{align*}
%         R_{F^{T}}(h_{n}) \to R^{*}_{F^{T}}
%     \end{align*}
%     Or (recall we are assuming 0-1 loss)
%     \begin{align*}
%         \int_{\mc{X}}\sum_{y \in \{1, \dots, k^T\}}\mbb{I}(h_n(x) \neq y)p(y)dF_X^T \to \int_{\mc{X}}\sum_{y \in \{1, \dots, k^T\}}\mbb{I}(h^*_T(x) \neq y)p(y)dF_X^T
%     \end{align*}
%     as $n \to \infty$. Without loss of generality, we assume all $x \in \mc{X}$ have positive density/probability and $p(y) > 0$ (simply throw out the points with zero probability/density). 
    
%     Since $R_{F^{T}}(h_{n}) \to R^{*}_{F^{T}} $, and $R^{*}_{F^{T}}$ is the infimum of the risk of all decision rules, and we are assuming $p(y|x)$ is uniquely maximized by some $y$, and all the points $(x, y) \in \mc{X} \times \{1, \hdots, k^{T}\} $ have positive density, then we must have that $h_{n} \to h_{T}^{*}$ pointwise. Otherwise, if for any point $x$ we have that $\lim_{n\to\infty}h_n(x) \neq h_T^*(x)$, then $\lim_{n\to\infty}R_{F^{T}}(h_{n}) > R^{*}_{F^{T}} $, contradicting our assumption. Thus $h_n \to h_T^*$ pointwise. 
    
%     Going back to task similarity, we thus have that
%     \begin{align*}
%         \lim_{n\to\infty} TS(F^T, F^S_n) & = \lim_{n\to\infty}\int_{\mc{X}}\mbb{I}(h_T^*(x) = h_n(x)\}dF^T_X \\
%         & = \int_{\mc{X}}\lim_{n\to\infty}\mbb{I}(h_T^*(x) = h_n(x)\}dF^T_X \\
%         & = \int_{\mc{X}}\mbb{I}(h_T^*(x) = h_T^*(x)\}dF^T_X \\
%         & = \int_{\mc{X}}dF^T_X \\
%         & = 1
%     \end{align*}
%     Where the interchange of the limit and the integral is justified by the dominated convergence theorem. Thus,
%     \begin{align*}
%          \lim_{n\to\infty} TS(F^T, F^S_n) = 1
%     \end{align*}
%     as desired.
% \end{proof}

% \begin{proof}
%     Let $ \mc{A}_{1}, \mc{A}_{2}, \hdots $ be a sequence of partitions such that $ \max_{A_{i_{n}}\in \mc{A}_{n}}  diam(A_{i_{n}}) \to 0 $ as $ n \to \infty $. Then any sequence any $(h_n)_{n = 1}^{\infty}$ such that $h_n \in \mc{H}_{\mc{A}_n}$ is a histogram rule. Let $F^T$ be an arbitrary distribution on $\mc{X}\times\{1, \dots, k\}$. Since histogram rules are universally consistent, we have that there must exist a specific sequence $(h_n)_{n = 1}^{\infty}$ such that $R(h_n) \to R^*$, a $n \to \infty$, where $R^*$ is the Bayes risk associated with $F^T$. Thus $(\mc{A}_n)_{n = 1}^{\infty}$ induces a consistent decision rule for $F^T$. By the previous theorem, $\lim_{n \to \infty}TS(F^T, F^S_n) = 1$ whenever $F^S_n \in \mc{F}_{\mc{A}_n}$, as desired.
% \end{proof}


% \section{Description of pairwise properties of XOR, Quads, R-XOR and F-XOR}\label{app:illustrative}


% 1. XOR and Quads share an optimal partition $ \mc{A}^{*} $. This means that the optimal partition aligner for both ``directions" maps a subspace to the set than contains just itself and the optimal labeler learns the bit flip that is the difference between the two distributions.

% 2. XOR and R-XOR are orthogonal distributions. For R-XOR to XOR, an optimal partition aligner maps a partition of XOR with patterns corresponding to class $ y $ to a set containing a partition of R-XOR with patterns corresponding to class $ y $. An optimal labeler can then map to either class 0 or class for each of the partitions. Since the optimal labeler is not unique for any of the partitions, the the adjustment labeler $ \pi' $ and the optimal labeler $ \pi^{*} $ are not equal on the entire space. Hence, the $ ATS $ is 0. This is similarly true for XOR to R-XOR.

% 3. XOR is adversarial for F-XOR but $ ATS $(XOR, F-XOR) = 1. For F-XOR to XOR, an optimal partition aligner maps each of the quadrants to its constituent ``quadrants within a quadrant" and the optimal labeler maps each of the labels for the ``quadrants within a quadrant" to the label of the quadrant. For XOR to F-XOR, an optimal partition aligner maps each of the ``quadrants within a quadrant" to its corresponding quadrant and the optimal labeler maps each of the quadrants to either to 0 or to 1. Since the optimal labeler can map to either 0 or 1 for each of the quadrants, the adjustment labeler and the optimal labeler are not equal on the entire space and so the $ ATS $ is 0. 

% 4. R-XOR is adversarial for F-XOR and $ ATS $(R-XOR, F-XOR) is neither 0 nor 1.  {\color{red} todo.}

% \section{Experimental Design}

% \textcolor{red}{Brandon.}
